# Supplementary material for: Scientific Spirit of Chien-Shiung Wu: From Quantum Entanglement to Parity Nonconservation
Source: arXiv:2504.16978 ancillary file (2025-04-23)
Supplement: Supplementary file 1 [file slides_of_the_presentation.pdf]

# Scientific Spirit of Chien-Shiung Wu: From Quantum Entanglement to Parity Nonconservation

Yu Shi

(Fudan University)

International Symposium Commemorating the  
110th Birth Anniversary of Chien-Shiung Wu  
Southeast University

2022.5.31.

Yu Shi, Scientific spirit of C. S. Wu: from quantum  
entanglement to parity nonconservation

# Overview of Chien-Shiung Wu's academic career and research work

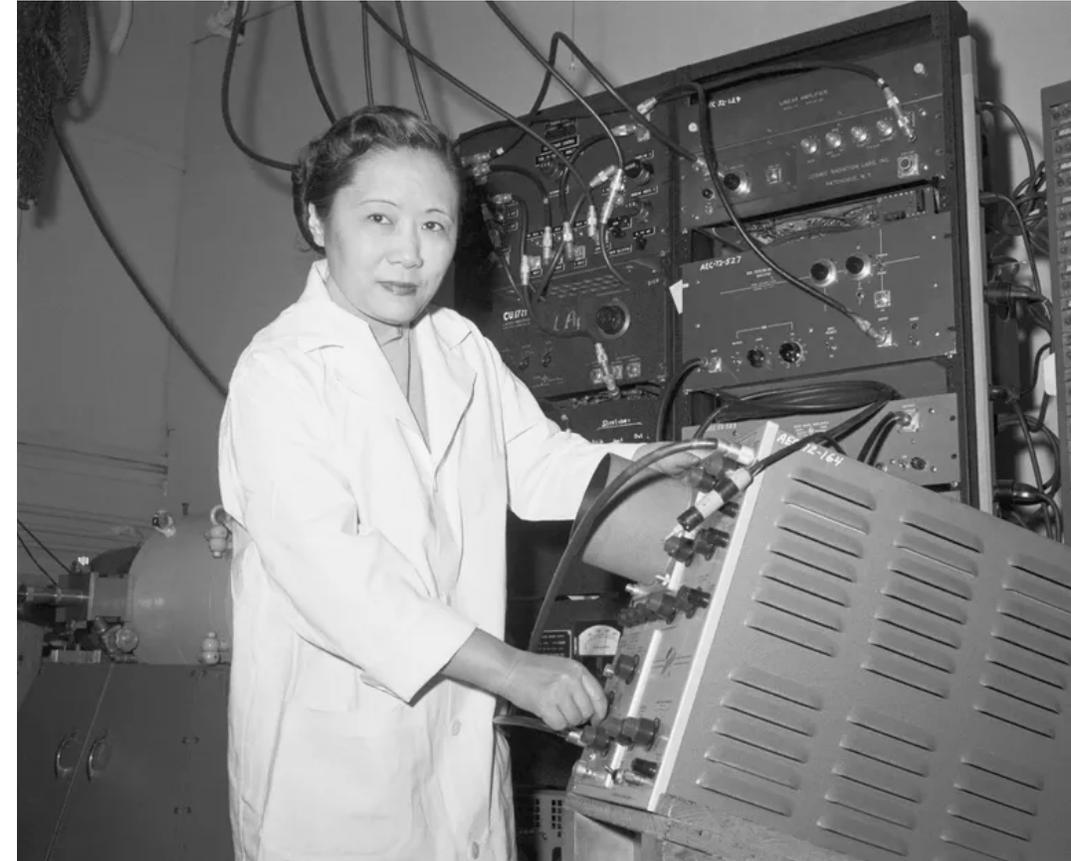

Yu Shi, Scientific spirit of C. S. Wu: from quantum entanglement to parity nonconservation

# China

- 1934, BS, Central University: Verification Bragg diffraction equations of X-rays in crystals, supervisor: Shih-Yuan Sze (PhD on nuclear spectroscopy, supervisor: Marie Curie).
- 1934-1935, Teaching Assistant, Chekiang University.
- 1935-1936, Institute of Physics, Academia Sinica (Shanghai), gas spectroscopy, supervisor: Z. W. Ku (PhD, University of Michigan, Supervisor: D. M. Dennison), China's first female doctoral degree.
- Fields Wu was initially exposed to, though not in nuclear physics, had much in common with her later field of radioactivity.
- Due to Ku's recommendation and advice, Wu was admitted by University of Michigan at her own expense with financial support from her uncle.
- En Route, Wu visited Dept of Physics at Univ of California, Berkeley, was deeply impressed, esp. by the cyclotron of Lawrence, learned of gender discrimination and there were too many Chinese students at Univ of Michigan. Successfully stayed at Berkeley (Ref: Wu Biography by Chiang).

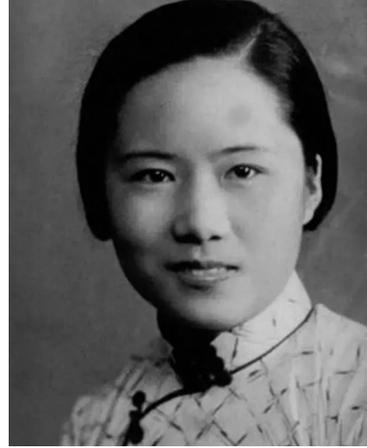

# PhD (1936-40) vs. Postdoc (1940-42), Berkeley

- 1938: Electron-excited **x-rays** from  **$\beta$  decay** of radioactive lead, advised by E. O. Lawrence.
  - The continuous x-rays excited by the beta-particles of P-15(32), Wu, CS, Mar 1941 | PHYSICAL REVIEW 59 (6) , pp.481-488 **Studied  $\beta$  decay at the beginning of career.**
- 1939-1942: Studied uranium fission products, esp. **radioactive xenon (identified two isotopes)**, using neutrons from **cyclotron**, advised by E. Segrè. Results on the neutron absorption section later contributed to Manhattan Project (atom bomb).
  - Some fission products of uranium, Segre, E and Wu, CS, Mar 1940 | PHYSICAL REVIEW 57 (6) , pp.552-552
  - Identification of two radioactive xenons from uranium fission, Wu, CS, Nov 1940 | PHYSICAL REVIEW 58 (10) , pp.926-926
  - RADIOACTIVE XENONS, WU, CS and SEGRE, E, **1945** | PHYSICAL REVIEW 67 (5-6) , pp.142-149
- 1940-1942: Studied **radioactive mercury** using **neutrons** from the cyclotron, with graduate student G. Friedlander.
  - Radioactive isotopes of mercury, Wu, CS and Friedlander, G, Nov 1941 | PHYSICAL REVIEW 60 (10) , pp.747-748
  - Radioactive isotopes of mercury, Friedlander, G and Wu, CS, Apr 1943 | PHYSICAL REVIEW 63 (7/8) , pp.0227-0234

# 1942-1948

- 1942-1943: Taught at Smith College
- 1943-1944: Taught at Princeton University
- 1944: Joined Columbia University and worked on the Manhattan Project.
- Work on the Manhattan Project (before 1945), continued for a few post-war years. Collaborators: [Dunning](#), [Rainwater](#), [Havens](#).  
**Significant contributions to Manhattan Project.** Some of the papers were for work done during the war, declassified and published after the war. [previously misunderstood as started after the war].
  - **Slow neutron effect of hydrogen and other elements, about 8 papers published in 1946-1948.**
  - **Sensitive Radiation Detector (detecting  $\beta$  electrons, photons, and other particles), about 7 papers were published in 1947-1948.**

# $\beta$ decay studies 1946-1956 (before parity Revolution)

- After the war, Wu systematically carried out long-term research on  $\beta$  decay and compared experiments with theories.
- From 1949 to 1956, Wu published about 53 papers on  $\beta$  decay (including a small number on electron capture), and became a leading expert on  $\beta$  decay (but was unfairly treated and remained an associate professor).
- Tsung-Dao Lee once said that in the field of  $\beta$  decay, no one can compare with Wu.
- Testing Fermi's  $\beta$  decay theory:
  - THE BETA-RAY SPECTRA OF CU-64, WU, CS and ALBERT, RD, 1949 | PHYSICAL REVIEW 75 (2) , pp.315-316
  - THE BETA-RAY SPECTRA OF CU-64 AND THE RATIO OF N+/N-, WU, CS and ALBERT, RD, 1949 | PHYSICAL REVIEW 75 (7) , pp.1107-1108
  - THE BETA-RAY SPECTRA OF CU-64, ALBERT, RD and WU, CS, 1949 | PHYSICAL REVIEW 75 (8) , pp.1286-1286
  - Chen Ning Yang: "Fermi's theory was proven correct! Wu became a leading scientist in the field of  $\beta$  decay experiments! "
  - The meticulousness of Wu's experiments, her skills of assembling and operating the instruments.

# Positronium and electron-positron annihilation

- 1950-1957, 6 papers were published on it.
- The first paper accurately tested the predictions of quantum electrodynamics. Meanwhile, quantum entanglement of photon polarization was realized:
- THE ANGULAR CORRELATION OF SCATTERED ANNIHILATION RADIATION, WU, CS and SHAKNOV, I, 1950 | PHYSICAL REVIEW 77 (1), pp.136-136

# 1957 Parity nonconservation

- In 1956, Tsung-Dao Lee and Chen-Ning Yang proposed that parity may not be conserved in weak interaction, and suggested several experiments.
- Wu collaborated with several low-temperature scientists to complete the polarized Co60 decay experiment, and found that the **parity is indeed not conserved**, which is a revolutionary breakthrough in nuclear and particle physics.
  - EXPERIMENTAL TEST OF PARITY CONSERVATION IN BETA-DECAY, WU, CS; AMBLER, E; HAYWARD, RW; HOPPES; HUDSON, RP, 1957 | PHYSICAL REVIEW 105 (4) , pp.1413-1415
  - FURTHER EXPERIMENTS ON BETA-DECAY OF POLARIZED NUCLEI, AMBLER, E; HAYWARD, RW; HOPPES, DD; HUDSON, RP ; WU, CS, 1957 | PHYSICAL REVIEW 106 (6) , pp.1361-1362

# Wu's papers after parity revolution

- 1957: A gas scintillation counter to detect slow neutrons.
- 1962-1985:  $\beta$  decay (about 16 papers), including double  $\beta$  decay.
- In particular, the theory of conservation of vector current was confirmed in 1963.
- 1973-1978: The Mössbauer effect of hemoglobin and other materials (about 15 papers).
- 1974-1984: Muon captures of exotic atoms and nuclei (about 23 papers).
- 1975: Positron and Negative Electron Couples and Annihilation (1 paper).
- 1976-1985: Nuclear orientation (about 6 papers).

# 1963 Vector Current Conservation

- EXPERIMENTAL TEST OF CONSERVED VECTOR CURRENT THEORY ON BETA SPECTRA OF B12 AND N12, LEE, YK; MO, LW and WU, CS, 1963 | PHYSICAL REVIEW LETTERS 10 (6) , pp.253。
- After the discovery of parity non-conservation, 3 groups proposed V-A theory (Universal Fermi Interaction) of weak interactions.
- Feynman and Gell-Mann proposed the assumption of conservation of vector current, which explained the equality of the coupling constants of different weak decays (e.g., nuclei and muons). They proposed that in nucleon renormalization, virtual  $\pi$  mesons also participate in weak interactions, resulting in the  $\beta$  decay coupling constant being unchanged.
- Gell-Mann pointed out that the conservation of vector current results in so-called "weak magnetism", similar to the difference between the magnetic moment between protons and neutrons in quantum electrodynamics (both values are 4.7). He suggested using the decays of B12 and N12 to test. Before Wu, experiments had been unsuccessful.
- In 1963, Wu Chien-Shiung and his student Y.K. Lee and L.W. Mo completed such experiments, confirmed the "weak magnetism", verified the conservation of vector current, and promoted the establishment of the unified electroweak theory.
- Wu: "The conserved vector current hypothesis for weak interactions has been confirmed experimentally and has served as a guiding principle for the modern gauge theory of strong and weak interactions, where it is predicted as a necessary consequence of vector gauge theory."

# Wu's Speech as President of the American Physical Society: The State of American Physics - 1976

- Recalled two famous addresses by Rowland, founder and first president of APS the end of 19<sup>th</sup> century (frustration about the backwardness of American physics at the time, but expressed hope for the future). Summarized the progress:
- Nuclear physics: nuclear charge distribution through electron scattering; protons scattered by nuclei; **nuclei absorbing pions and jumping to rotational highly excited states; muon atoms verifying QED**; parity nonconservation in nuclear scattering; heavy ion collisions to study rapidly rotating nuclei; nuclear disintegration.
- Cosmic rays: possible magnetic monopoles.
- Synchrotron radiation used in biology, solid state physics, chemistry.
- Biophysics: addition of heavy atoms to protein molecules, X-ray diffraction; about hemoglobin, synchrotron radiation and the **Mössbauer spectra from Columbia** revealed differences in various situations.
- Solid State Phys: measuring local magnetic fields in solids with muons; the field is active.
- Particle physics: muons  $g-2$  experiment tested lepton universality; positronium; charmonium ( $J/\psi$ ).

# Electron-positron annihilation and quantum entanglement

Yu Shi, Scientific spirit of C. S. Wu: from quantum entanglement to parity nonconservation

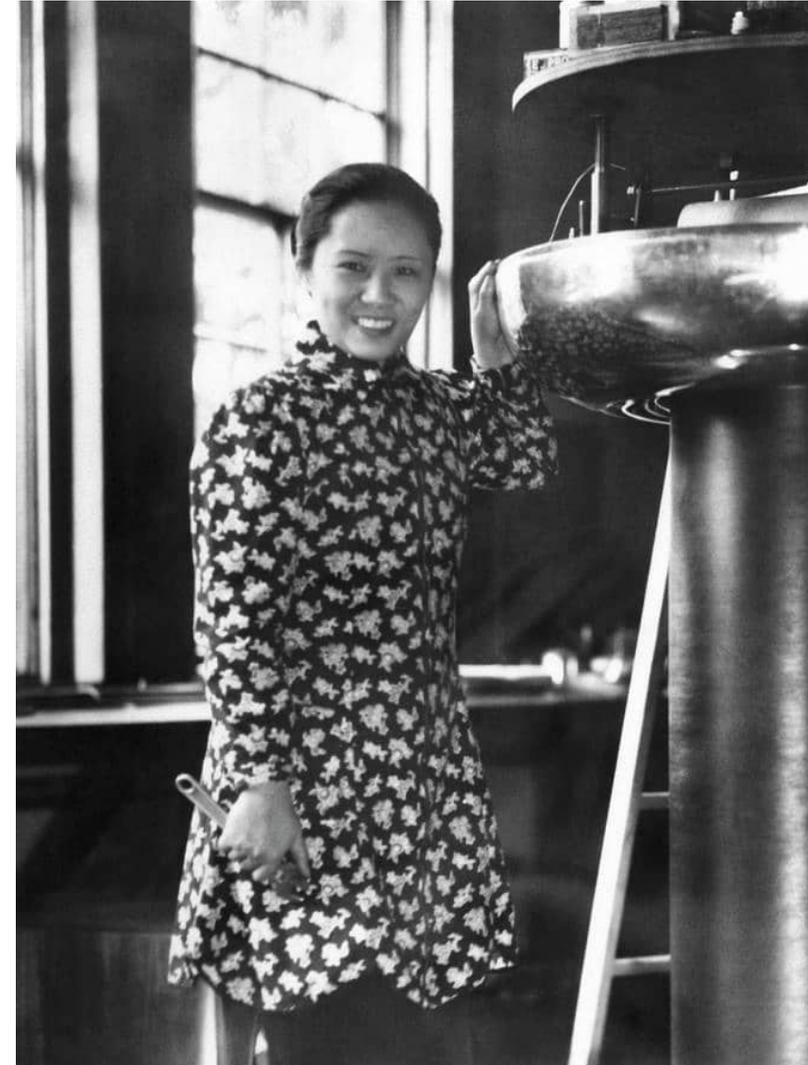

# Wu, Shaknov, 1950

## The Angular Correlation of Scattered Annihilation Radiation\*

C. S. WU AND I. SHAKNOV

*Pupin Physics Laboratories, Columbia University, New York, New York*

November 21, 1949

- Test QED, Wheeler proposed to study electron-positron annihilation. Further calculations by Ward-Price, and by Snyder-Pasternack-Hornbostel.
- Two photons created in electron-positron annihilation, polarizations are always perpendicular, scattered by electrons respectively.
- For different scattering angles, measure the asymmetries between the two situations of moving directions being perpendicular and parallel.
- Maximum=2.85, when the scattering angle=82°
- The polarization determines the scattering distribution.
- Previous experiments not satisfactory.
- Sensitivity of the  $\gamma$  detector by Wu and Shaknov was 10 times that of previous ones.
- Positron source Cu64 was activated by deuterium bombardment in Columbia cyclotron.
- Result:  $2.04 \pm 0.08$ . (Theory: 2.00)

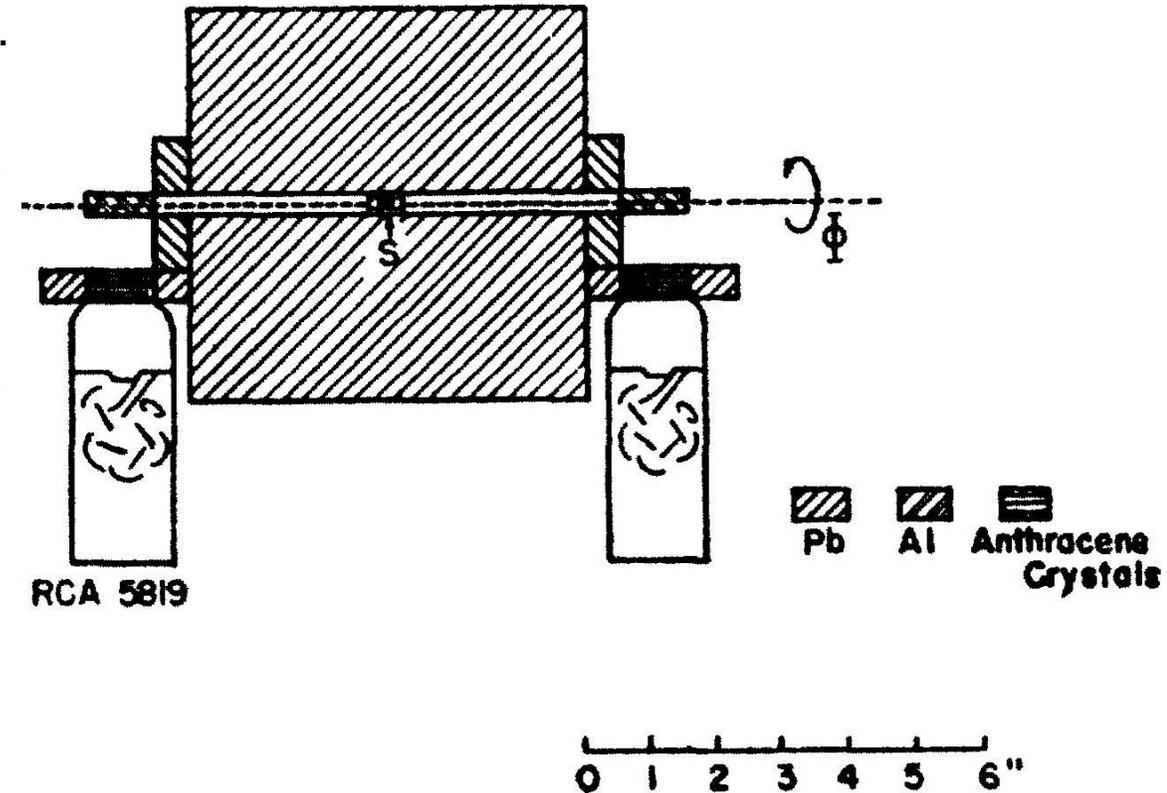

FIG. 1. Schematic diagram of experiment.

Yu Shi, Scientific spirit of C. S. Wu: from quantum entanglement to parity nonconservation

# Quantum Entanglement

- In 1935, Einstein-Podolsky-Rosen demonstrated the conflict between local realism and quantum mechanics using quantum entangled states. They claimed that quantum mechanics is incomplete.
- In the same year, Schrödinger coined quantum entanglement, noting that it is a characteristic of quantum mechanics.
- In 1957, Bohm-Aharonov noted that Wu-Shaknov achieved photon polarization correlation (Bohm-Aharonov did not use the word "entanglement"). They proved that the non-entangled state could not give the experimental results of Wu-Shaknov.
- For the first time, Wu-Shaknov experimentally achieved a clearly spatially separated quantum entangled state. In terms of expression of today:

$$\frac{1}{\sqrt{2}} (|h\rangle|v\rangle - |v\rangle|h\rangle)$$

Yu Shi, Scientific spirit of C. S. Wu: from quantum entanglement to parity nonconservation

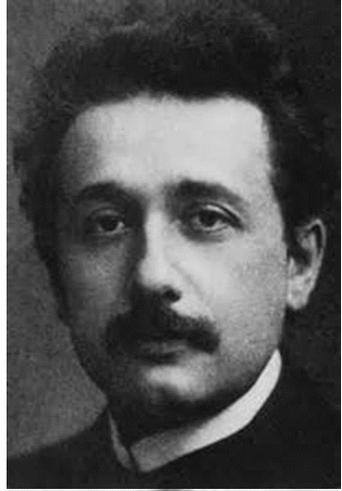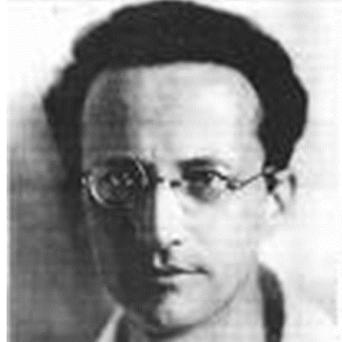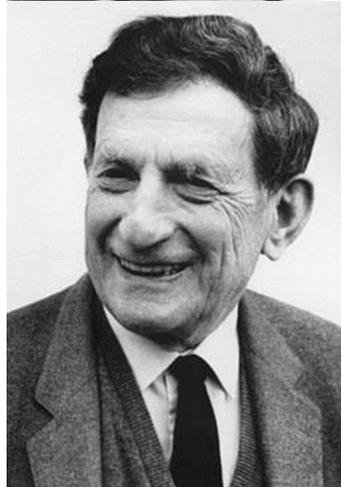

# 1975, Wu's group attempted to test Bell's inequality

- In 1964, Bell proposed the inequality satisfied by local realism (hidden variables).
- Quantum entangled states violate Bell's inequality, but polarization needs to be measured in a direction that is neither parallel nor perpendicular.
- In 1950 Wu-Shaknov experiment, the azimuth angles of the two photons detected were always perpendicular.
- In 1975, Chien-Shiung Wu and his students Kasday and Ullman measured **the coincidence probability of two photons in a wide range of polar and azimuthal angles**.
- ANGULAR-CORRELATION OF COMPTON-SCATTERED ANNIHILATION PHOTONS AND HIDDEN VARIABLES, KASDAY, LR; ULLMAN, JD, d WU, CS, 1975 | NUOVO CIMENTO B 25 (2) , pp.633-661.
- The results are consistent with the entangled state and contradict the non-entangled state.
- However, it cannot be used to prove that Bell's inequality is violated, because local realism can also calculate Compton scattering, and it cannot explicitly lock the direction of photon detection and polarization in a certain direction.
- Here are **high-energy photons**, which are not easy for direct polarization measurements (can destroy polarizers). The polarization of low-energy photons can be measured directly with polarizers.
- **Contemporary quantum information science is booming by using the entangled states of low-energy photons and other agents.**

# Parity nonconservation

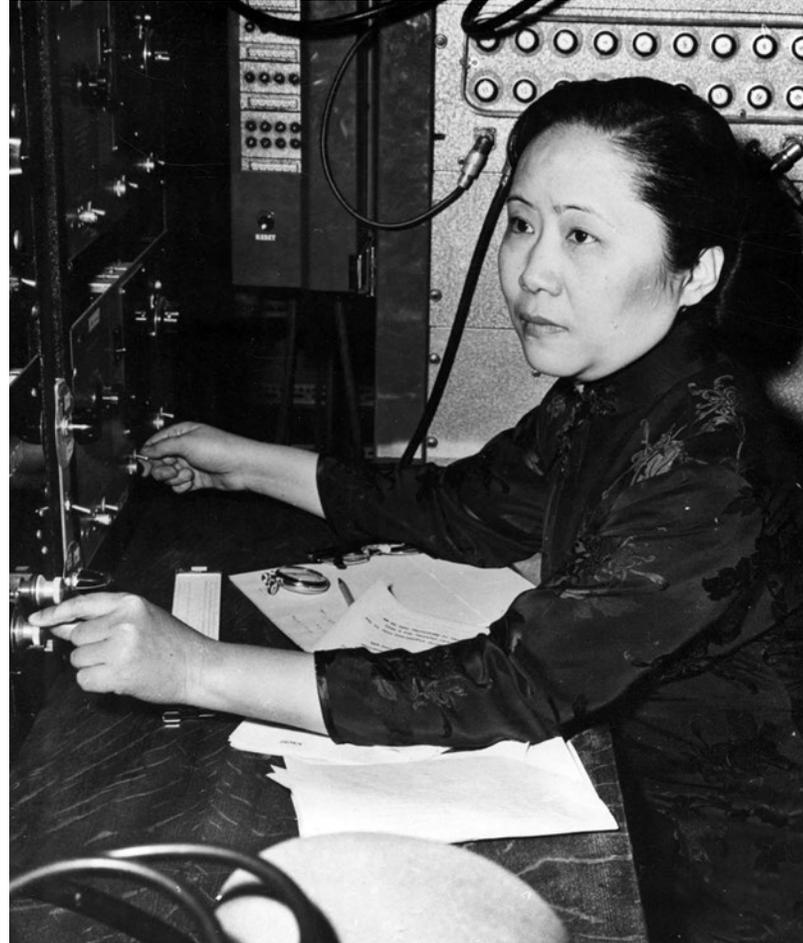

Yu Shi, Scientific spirit of C. S. Wu: from quantum entanglement to parity nonconservation

# First half of 1956

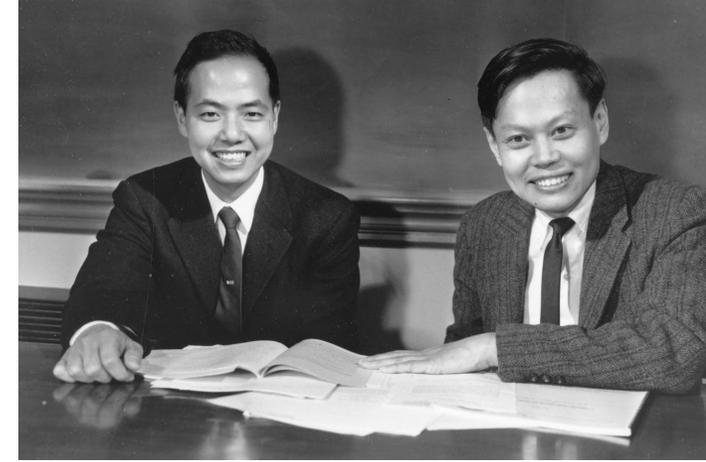

- Chen-Ning Yang (IAS Princeton and Brookhaven Lab) and Tsung-Dao Lee (Columbia University) extended the  $\theta$ - $\tau$  puzzle to the general problem of weak interactions, studying the possibility that "the parity is conserved in strong and electromagnetic interactions, but may not be conserved in weak interactions", and focused on the decay process dominated by weak interactions. Among these decays, the most studied is  $\beta$  decay. Previous calculations were based on parity conservation. They took into account the possibility of parity nonconservation and calculated the results of various experiments.
- During this period (May), Lee went to talk to Chien-Shiung Wu, an expert on  $\beta$  decay. Wu lent Lee the anthology edited by Siegbahn.

# Polarized Co60

- Yang-Lee calculations showed that if parity is not conserved, the results not involving pseudoscalars remain the same as if parity is conserved, so those experiments cannot prove whether parity is conserved in weak interactions. But results concerning pseudoscalars are different.
- No one had measured pseudoscalars (an exception was unearthed later in 1959). Polarized nuclei can be used to measure helicity, a pseudoscalar.
- Goldhaber of Brookhaven told Yang that nuclei had been polarized by low temperature techniques.
- Lee discussed with Chien-Shiung Wu and said that the  $\beta$  decay of polarized nuclei can be used to measure helicity and test whether the symmetry is conserved.
- Wu suggested polarizing Co60 nuclei at low temperatures. She had been following this technology for several years.

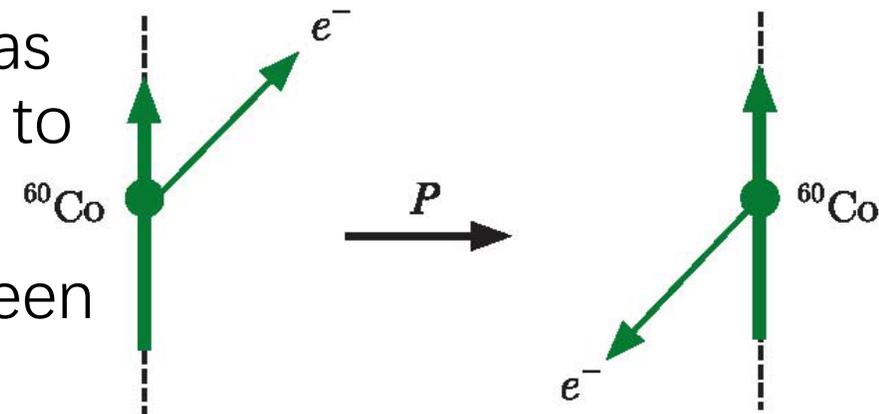

# Preparation for Wu experiment

- Regarding it as the golden opportunity, Wu decided to do this experiment herself: **even if parity is indeed conserved, an upper limit of the parity violation can be given.**
- Wu considered that although it was unlikely that the parity is not conserved, it should be tested before anyone else. For this reason, Wu abandoned the travel plan to East Asia.
- The new version of the nuclear data changed the Co60 spin, and if it is correct, it is not suitable. Did an experiment with an assistant to confirm that it should not be changed.
- Learned techniques from the cryogenic group in the department.
- 6.4., called E. Ambler (Bureau of Standards), inviting cooperation. [Ambler was from the Oxford group that had polarized Co60]
- June-July, tested  $\beta$  detectors, considered a lot of questions. [Lee-Yang's paper was submitted on June 22]
- 7.24, called Ambler again. A few days later, Ambler sent Wu a rough diagram of the cryostat, then was vacation for two weeks.
- August, studied the effect of magnetic field on  $\beta$  counting, and the scattering of  $\beta$  particles by cerium magnesium nitrate crystals (CMN, used to polarize Co60).

# Wu experiment

- Mid-September, Wu met with Ambler for the first time. Hudson, Hayward, Hoppes joined.
- The third time to Washington DC, Wu brought two CMN crystals with Co60 (for polarizing Co60). Later, a large number of CMN crystals were needed, which Wu and his assistant grew at Columbia.
- **Mid-December, an asymmetrical signal was seen for the first time, and it was large.** However, it was believed that systematic verification was needed before announced to the public.
- One Thursday, Wu met Lee and Yang and told them that **the effect was large and reproducible, but it was only a preliminary result.**
- After a week, other possible factors began to be ruled out.
- Wu later recalled: returned to the NY train station on Christmas Eve, called Lee and told him that the asymmetric parameter was almost -1.
- **This showed that the neutrino two-component theory by Lee-Yang in summer is correct. (anti)neutrinos are always (right) left-handed. (submitted on 1.10.)**
- **According to the analysis by Lee-Oehme-Yang, the results also imply that CP symmetry is also violated broken. (submitted on 1.7.) [Wu experiment promoted Lee-Yang theoretical work]**

Yu Shi, "Scientific spirit of C. S. Wu: from quantum entanglement to parity nonconservation"

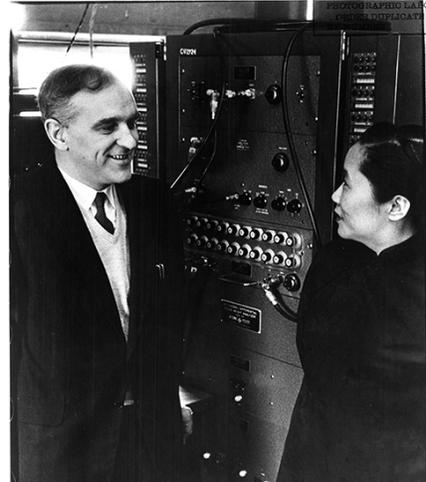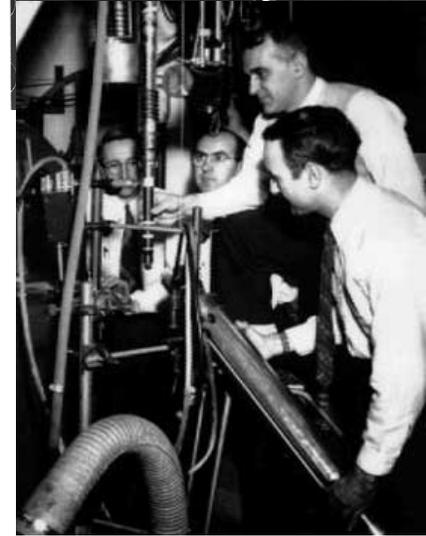

# $\pi$ - $\nu$ - $e$ decay

- Lee-Yang paper discussed several experiments that can be done, including Co60 and  $\pi$ - $\mu$ - $e$ , to test whether parity is conserved in weak interactions.
- Nevis lab affiliated with Columbia often produces  $\pi$ - $\mu$ - $e$ . When Yang met Lederman of Nevis in Brookhaven, Yang suggested Lederman use  $\pi$ - $\mu$ - $e$  to test parity conservation. Lederman was not willing.
- By the time of Christmas, the message of Wu experiment had spread.
- 1.4., Lee revealed during the regular Friday lunch that the parity violating effect in Wu experiment was great. Lederman began  $\pi$ - $\mu$ - $e$  experiment with Garwin and Weinrich that night. The experiment was simple. In the early hours of Tuesday (8th), Lederman called Lee: "The law of parity is dead. "

# The result of the Wu experiment was confirmed

- Wu experiment promoted Lee-Yang theory and  $\pi$ - $\mu$ -e experiment, but the conclusion of Wu experiment has not yet been conclusively confirmed!
- 1.2-9, the most intense stage of experimentation of Wu group.
- Though Garwin-Lederman-Weinrich results of  $\pi$ - $\mu$ -e were out (Wu was not very happy), Wu group **did not let up until the results were fully confirmed**. On the 9th, at 2:00, the parity violation was celebrated.
- 1.15, Columbia press conference, and the two papers were submitted. Next day, NYT headline. Published back to back on 2.15 (headed by Wu experiment)..
- $\pi$ - $\mu$ -e by Friedman-Telegdi at Chicago was published on 3.1.

## Experimental Test of Parity Conservation in Beta Decay\*

C. S. WU, *Columbia University, New York, New York*

AND

E. AMBLER, R. W. HAYWARD, D. D. HOPPES, AND R. P. HUDSON,  
*National Bureau of Standards, Washington, D. C.*

(Received January 15, 1957)

Yu Shi, Scientific spirit of C. S. Wu: from quantum entanglement to parity nonconservation

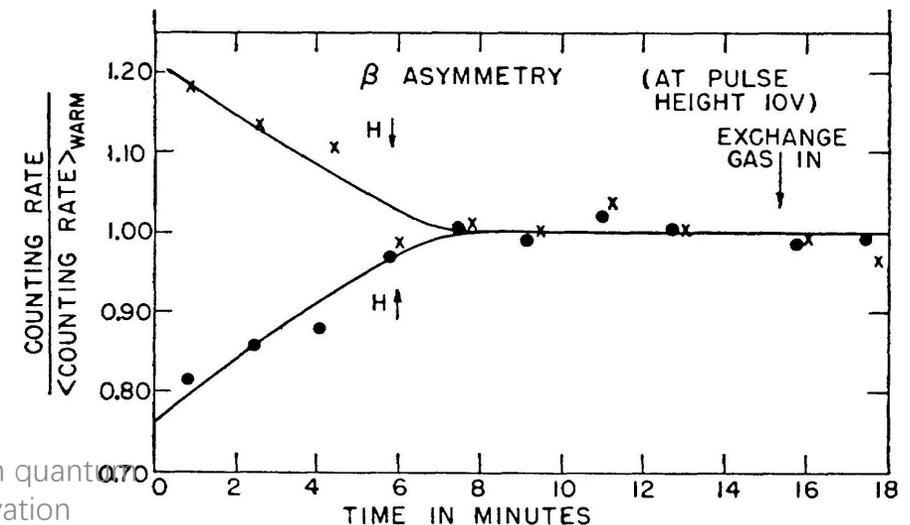

# Wu group discovered parity nonconservation in weak interactions

- Yang and Lee noted after detailed calculation: there had been no experiments proving whether the parity is conserved in weak interactions. They pointed out several types experiments to test whether parity is conserved in weak interactions.
- However, they did not say whether parity must be nonconserved (at that time, they also proposed parity doublet with parity conservation to solve  $\theta$ - $\tau$  puzzle). Whether parity is conserved or not was up to experimental test.
- For a long time, parity conservation had an intuitive appeal, and was regarded as natural, sacred, and very useful. Therefore the paper by Yang and Lee was **generally despised, dissented, and even ridiculed.**
- But Wu Chien-Shiung Wu decided to do a  $\beta$  decay testing experiment with  $\text{Co}60$ .
- **Wu experiment showed that parity is indeed nonconserved in weak interactions, causing a huge shock in the entire physics community.**
- One of the most important experiments in physics of the 20th century.
- Cronin: **"The great discovery of Chien-Shiung Wu has opened the golden age of particle physics."**

# Chien-Shiung Wu: A great experimental physicist

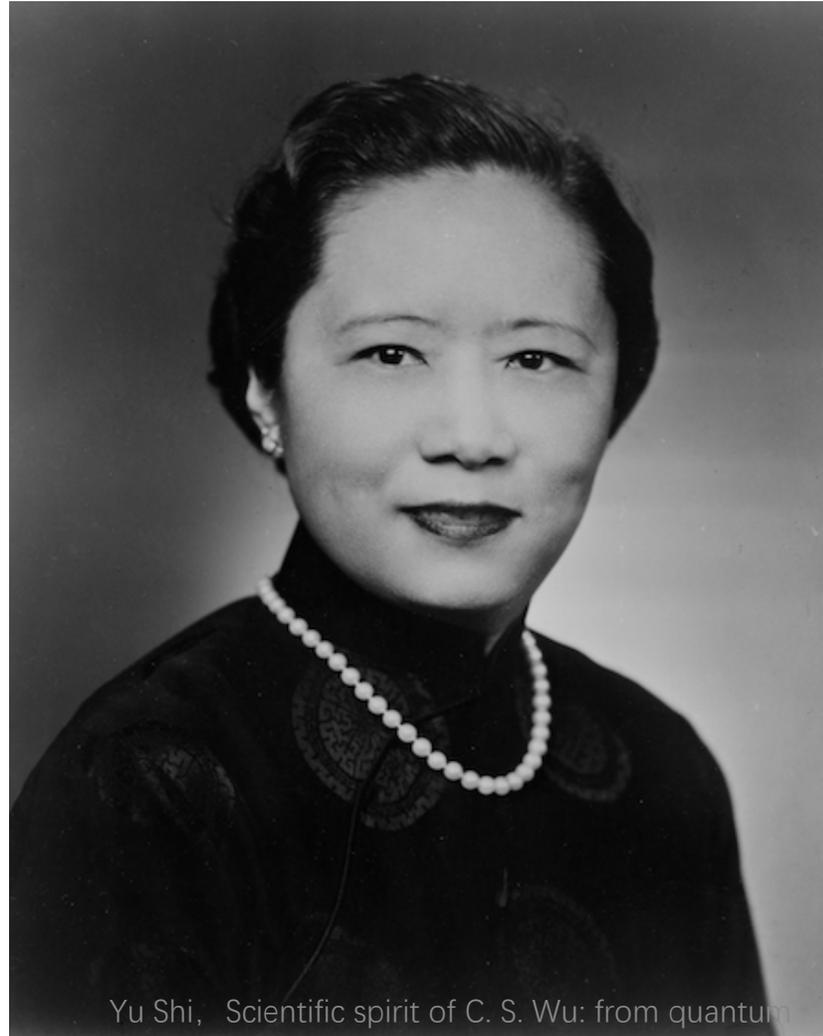

Yu Shi, Scientific spirit of C. S. Wu: from quantum entanglement to parity nonconservation

# Chien-Shiung Wu: A great experimental physicist

- Intelligent, quiet, diligent, hardworking, focused, **undaunted by difficulties, dedicated to science**. (at her childhood, her father said: "Don't be afraid of difficulties, work hard, and move forward")
- Accurate experiments. Elements **of Chinese girls' specialties, and embodiment of the scientific integrity**.
- Research areas and achievements are closely related to **years of experiences and expertise**.
- Attach importance to the development of experimental techniques and instruments, but also to physical significance, master important theories, and verify theories with experiments.
- Her experimental work has great theoretical significance, e.g. the verification of Fermi theory, the prediction of quantum electrodynamics on photon coincidence and quantum entanglement, parity nonconservation, vector current conservation, and double  $\beta$  decay.
- Whether it's overthrowing or verification, do it.
- **I think the most valuable is: prioritizing scientific rigor over competition and honor, even when priority and merit are at stake** (indeed there was some damage, although publication is respected, may be one of the factors in missing the Nobel Prize). Another manifestation of her scientific spirit.

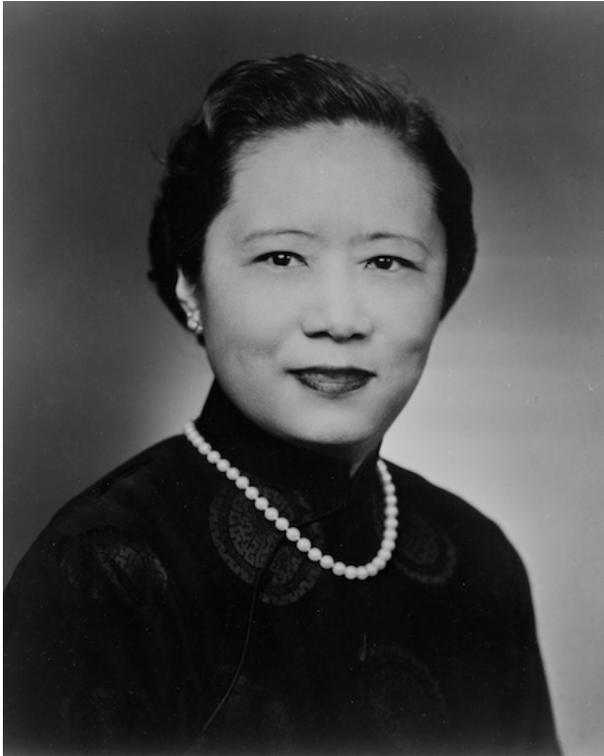

Yu Shi, Scientific spirit of C. S. Wu: from quantum entanglement to parity nonconservation

- Chen Ning Yang: “The research works of Ms Chien-Shiung Wu were well known for their **precision and accuracy**. But her great success was down to another more fundamental reason: in 1956, people did not want to do experiments to test parity conservation. Why was she willing to do this such a difficult experiment? Because she had the **penetrating perception** that even if parity conservation is not overthrown, this fundamental law of nature must be tested. Here resides her greatness.”
- Chen Ning Yang: “I once said that there are three necessary conditions for success in scientific research: **Perception, Persistence, and Power**. Chien-Shiung Wu satisfied all these three conditions. Her experiment on parity nonconservation met with many difficulties……The most important thing was her vision.”

- Tsung-Dao Lee: “She was **one of the most outstanding physicists of the 20th century**, who made great achievements in experimental physics research and played an extremely important role in advancing the development of contemporary physics.”
- Tsung-Dao Lee: “When Madam Curie passed away, Albert Einstein once wrote, ‘At a time when a towering personality has come to the end of her life, let us not merely rest content with recalling what she has given to mankind in the fruits of her work. It is the **moral qualities** of its leading personalities that are perhaps of even greater significance for a generation and for the course of history than purely intellectual accomplishments ... **Her strength, her purity of will ... her objectivity, her incorruptible judgment**, all these were of a kind seldom found **joined** in a single individual ... Once she had recognized a certain way as the right one, she pursued it without compromise and with extreme tenacity.’ I think that in remembering Chien-Shiung Wu, it is only fitting that we apply to her the words of Einstein praising Madame Curie.”

- The scientific life of Chien-Shiung Wu is situated in the context of 20th century history of China and the world.
- E. Segrè: “This trio of Chinese physicists shows what China’s future contribution to physics could be if that great country overcomes the period of revolutionary convulsions and resumes its historic role as one of the leaders of civilization, as witnessed by the early European travelers, to their astonishment.”
